# Supplementary material for: When LLM Rationales Become User-Facing: Effects on Trust Perception, Decision-Making, and Gaze Behaviors
Source: arXiv:2606.25489 source file (2026-06-24)
Supplement: Supplementary file 1 [file appendix.tex]

\clearpage
\onecolumn

% ====================================================

\begin{appendices}

\section{Analysis Results of the Eye Tracking (Gaze) Measure}
\label{appendix: study_procedure}

\end{appendices}

\setcounter{table}{0} % Reset table counter
\setcounter{figure}{0} % Reset table counter

\input{tables/lab_gaze}

% ===================================================
